# Supplementary material for: Kernel Debiased Plug-in Estimation: Simultaneous, Automated Debiasing without Influence Functions for Many Target Parameters
Source: arXiv:2306.08598 source file (2024-06-02)
Supplement: Supplementary file 1 [file appendixA.tex]

% \lemmaexpension*

This expansion plays a significant role in motivating current estimation methods, such as \cite{van2006targeted} and \cite{bickel998}, and it also plays a crucial role
% plays a significant role 
in our method as well. We provide the proof for this expansion below:

\begin{proof}[Proof of Lemma~\ref{lemma:expension}]
We begin by revisiting a few simple results
% We first recall simple results 
that enable this form of expansion:
\begin{enumerate}[label=\textbf{L.\arabic*}]
    \item\label{l1} 
    By defining $h = p^*/\h{p} -1$, we get that $h$ is mean zero under $\h P$:
\[\h Ph = \int \left[\frac{p^*}{\h p} -1\right] d\h{P} = \int \left[\frac{p^*}{\h p}-1\right] \h{p} \ d\lambda = 1-1 = 0.\]
    Furthermore, if $f$ is an integrable function with respect to measure $P^*$, then:
    % we have that:
    \[
    \h{P}[f(1+h)] = \int f \times (p^*/\h p) \ d\h{P} = P^*[f]. 
    \]
    \item \label{l2}
    Since $P^*$ is absolutely continuous with respect to $\h P$, we have that
    $P_{\epsilon=1, h} = P^*$:
        \[
            p(\e=1|h) 
            =
            (1 + p^*/\h{p}-1)\h{p} = p^* 
            %\implies P_{\epsilon, h}|_{\e = 1} = P^*  
        \]
    \item\label{l3} 
    Recall by the definition of $\Tcal_{{P}}$, ${P}[\phi_{{P}}] = 0$ for any $P$ in the model.
\end{enumerate}
Consider the first-order distributional Taylor expansion of pathwise differentiable $\psi$ along $\hat p_{\e,h}$ around $\hat p$ (i.e., $\e = 0$); note that the remainder term is defined by this expansion:
\begin{align}
    -[ \psi(\h P) - \psi(P^*) ]
    &= 
    \frac{
      \psi(P_{\e, h})- \psi(\h P)
    }{
      \e
    }\big|_{\e=1} 
    %&\text{(by \ref{l2})}
    \nonumber
    \\
    &\eqqcolon
    D_{\h P} \psi [h] + R_2(P^*, \h P)
    %&\text{(von-Mises Expansion)}
    \nonumber
    \\
    &= 
    \h P[\phi_{\h P} h] + R_2(P^*, \h P) 
    %&\text{(Reisz Representation Identity for $\phi_{\h P}$)}
    \nonumber
    \\
    &= 
    \h P[\phi_{\h P} h] -\h{P}[\phi_{\h P}] + R_2(P^*, \h{P}) 
    %&\text{($\h{P}[\phi_{\h P}]=0$ by \ref{l3})}
    \nonumber
    \\
    &=
    \h P[\phi_{\h P}(1+h)] + R_2(P^*, \h{P})
    \nonumber
    \\
    &= 
    P^*[\phi_{\h P}] + R_2(P^*, \h P) 
    %&\text{(by \ref{l1})}\label{eq:expansion}
    \label{eq:vonMises}
\end{align}
Then, we subtract the following zero term in our expansion %in Line~\eqref{eq:expansion}:
\begin{align*}
    &\PP_{n}(\phi_{P^*}) - \PP_n(\phi_{\h P}) + (\PP_n - P^*)(-\phi_{P^*}) + \PP_n(\phi_{\h P})
    %\\
    %&=
    %\underbrace{\PP_{n}(\phi_{P^*}) - \PP_{n}(\phi_{P^*})}_{= 0} 
    %+
    %\underbrace{\PP_n(\phi_{\h P}) - \PP_n(\phi_{\h P})}_{=0} 
    %+
    %\underbrace{P^*(\tilde \psi_{P^*})}_{=0 \ \text{by \ref{l3}}}
    .
\end{align*}
Collecting terms, multiplying by $-1$ and setting $R_2(\h P, P^*) = -R_2(P^*,\h P)$ leads to:
\begin{align*}
    & \psi(\h P) - \psi(P^*) 
    \\
    &\qquad =
    -P^*[\phi_{\h P}] + R_2(\h P,P^*) 
    +
    \Big[
      \PP_{n}(\phi_{P^*}) - \PP_n(\phi_{\h P}) 
      +
      (\PP_n - P^*)(-\phi_{P^*}) + \PP_n(\phi_{\h P})
    \Big]
    \\
    &\qquad =
    \PP_n\phi_{P^*} - \PP_n\phi_{\h P} + (\PP_n - P^*)\big[\phi_{\h P} - \phi_{P^*}\big]+ R_2(\h P, P^*)
    \tag{\ref{eq:asyExpansion}}
    .
\end{align*}
\end{proof}
