# Supplementary material for: Kernel Debiased Plug-in Estimation: Simultaneous, Automated Debiasing without Influence Functions for Many Target Parameters
Source: arXiv:2306.08598 source file (2024-06-02)
Supplement: Supplementary file 2 [file appendixC.tex]

% \textcolor{blue}{For those wondering why this section is here, Yaroslav and I are trying to work backward to flesh out the necessary conditions for \ref{app:proofs}}. \textcolor{blue}{We can merge these sections b, c as written currently to maintain simulations being in d.}

To provide an explicit example of Theorem \ref{thm:main}, we turn our attention to estimating $\psi_{\ATE}(P^*)$ using the mean-zero Gaussian kernel, under the set-up of our simulations provided in Section \ref{sec:sims}. To ease notation, we denote the conditional regression function as $Q_P(a,x)\coloneqq P(Y=1|A=a, X=x)$, and the propensity score function as $g_P(x)\coloneqq P(A=1|X=x)$. We intentionally denote the
% note that denoting the 
conditional regression function as $Q_P$ to emphasis that, 
% is intentional, as
% in our simulation set-up,
we only perturb the conditional regression function in our simulation set-up. 
To ease exposition,
we denote
% We provide both 
the form of $\psi_{\ATE}$
% , which we denote 
as $\psi$, and its corresponding influence function as $\phi_{P}$. In particular,
% below: 
% 
% might be easier to read first line with Q's inside
\begin{align}\label{eq:ate_if}
    \psi(P) &= P_X[Q_P(1,X)-Q_P(0,X)]\\
   \phi_P(Y,A,X) &=
   \left(\frac{A}{g_P(X)}-\frac{1-A}{1-g_P(X)}\right)
   (Y-Q_P(A,X)) 
   + (Q_P(1,X)-Q_P(0,X))-\psi(P). 
\end{align}
Under the conditions of Assumption \ref{assump:S3} and \ref{assump:S4}, we analyze our estimator using the expansion in Lemma \ref{lemma:expension}:
\begin{align}
    \psi(P_n^\infty) - \psi(P^*) = \PP_n\phi_{P^*} \underbrace{- \PP_n\phi_{P_n^\infty} + (\PP_n - P^*)\big[\phi_{P_n^\infty} - \phi_{P^*}\big]}_{(a)=\text{``pseudo-empirical process term''}}+ \underbrace{R_2(P_n^\infty, P^*)}_{(b)=\text{second-order remainder}}.\label{eq:ate_theory_expansion}
\end{align}
To obtain an asymptotically normal, efficient estimator, we need term $(a)$, a "pseudo-empirical process term", and term $(b)$, the second-order remainder, to vanish at an $o_{P^*}(1/\sqrt{n})$ rate. This section is organized as follows. First, we provide alternative conditions that ensure the $o_{P^*}(1/\sqrt{n})$ convergence rate, while assuming Assumptions \ref{assump:S3}, \ref{assump:S4} hold.  We then show how these alternative conditions (namely, Assumption \textbf{D3}) are sufficient for guaranteeing the $P^*$-Donsker conditions required for the convergence of the pseudo-empirical process term. By leveraging the asymptotic expansion of Lemma \ref{lemma:expension}, we explicitly show how our assumptions result in the desired limiting distribution. 

%In this section, we provide alternative conditions that ensure the high-level conditions of Assumptions \ref{assump:empprocess}, \ref{assump:secondorderremainder}, \ref{assump:S5} hold. We also provide a discussion of Assumptions \ref{assump:S3} and \ref{assump:S4}, demonstrating their technical role in Theorem \ref{thm:main}'s results. 

%We illustrate the assumptions outlined in 
% To make the assumptions in
%Theorem~\ref{thm:main}
%in the ATE case, 
% more concrete, 
% we provide 
% more specific
% conditions for the ATE case, 
%organizing them based on their respective use cases.
% , separating these assumptions by their use case. 
%In particular, we focus on Assumptions $\textbf{\textit{\ref{assump:secondorderremainder}, \ref{assump:S5}}}$, and $\textbf{\textit{\ref{assump:empprocess}}}$, which depend heavily on the  the target parameter $\psi$ and our model class $\Mcal$. We assume all other assumptions (i.e., $\textbf{\textit{S\ref{assump:S3}, S\ref{assump:S4}}}$) hold. 

\subsection{Alternative Conditions for  Assumptions \ref{assump:empprocess}, \ref{assump:secondorderremainder}, \ref{assump:S5}}\label{c:assumptions}
% kyra: rephrasing the below sentence
% Let there be an event $\Omega$ such that $P^*(\Omega)=1$.
% \kyra{it would be much better to define $\Omega$ explicitly. It seems unnecessary to define $\Omega$ as the general event here since we want w to be an n-sample realization
% In addition, it is a bit weird to use w to denote both an index and an n-sample realization.}

%ym: what is the role of \Omega? If it is not used in the conditions of this section, it should not be introduced.
Let $\Omega$ be the collection of all events $w$ (i.e. realizations of the data or sample paths) such that $P^*(\Omega) = 1$ as $n \rightarrow \infty$. For all $w \in \Omega$, we assume the following conditions hold:
\begin{enumerate}
    \item[\textbf{D1}] Appropriate rates of convergence for $P_n^0, P_n^\infty$:
    \begin{itemize}
        \item $\|g_{P_n^0} - g_{P^*}\|_{L_2(P^*)} = o_{P^*}(n^{-1/4})$;
        \item $
        \|Q_{P_n^\infty} - Q_{P^*} \|_{L_2(P^*)} = o_{P^*}(n^{-1/4})$.
    \end{itemize}
    \item[\textbf{D2}] Boundedness of $g_{P_n^0}$: We assume that $g_{P_n^0}$, our propensity score estimate, is bounded away from 0 by an absolute constant $c$, i.e., $c \leq g_{P_n^0(w)} \leq 1-c$ for all $x \in [0,1]$ as $n \rightarrow \infty$. 

    %\ym{boundedness abouve and below?}
    %\ym{I would emphasize that these bound must hold univormly accross the realizations of the data}

    % \kyra{the positivity assumption?} \brian{this is slightly different, as it's talking about the bound on our estimate $g_{P_n^0}$. However, if we assume positivity, and that $g_{P_n^0}\rightarrow g_{P^*}$ (consistency) [which we do], then positivity should be enough asymptotically!}
    %% Kyra: I see, you can decide whether to include the sentence below. I commented it out currently.
    
    %\item[\textbf{D3}] 
    % We estimate $g_{P_n^0}(\omega)$ and $ Q_{P_n^0}(\omega)$, such that they fall into a $P^*$-Donsker class. 
    %The initial estimates $g_{P_n^0}$ and $ Q_{P_n^0}$ are  continuously differentiable with respect to $\Xcal$, with partial derivatives that satisfy the following for some constant $M < \infty$ over all fixed $(Y,A)\in \{0,1\}^2$: 
    %\[\int_0^1 |\frac{\delta}{\delta x}g_{P_n^0}|dx \leq M,\quad\quad \int_0^1 |\frac{\delta}{\delta x}Q_{P_n^0}|dx \leq M.\]
    
    % \kyra{will continue from here.}
    %ym: $k$ is used to denote kernel as function of one variable
    % will fix notation, got it!
    \item[\textbf{D3}] We assume (1) $\sup_{O \in \Ocal} |p^*(O)/p_n^\infty(O)| \leq c$ for some constant $c$ as $n \rightarrow \infty$, and (2) there exists a sequence $\{h_j\}_{j=1}^\infty \subset \Hcal_{P_n^\infty}$ that satisfies both of the following conditions:
    \begin{itemize}
        \item $\|h_j - \phi_{P_n^\infty}\|_{L^2(P_n^\infty)} \rightarrow 0$ as $j \rightarrow \infty$;
        \item There exists $j_1 \in \NN$ such that $\int_0^1 |\frac{\delta}{\delta x}h_j| dx \leq M $ for some $M < \infty$ for all $j \geq j_1$. 
    \end{itemize}
    %Continuous differentiability of $K_P$: Let $\ell$ be the number of iterations for convergence. For all $j \leq \ell$, $n \in \NN$, we assume that $K_{P_n^j}$ is twice continuously differentiable with respect to $(x,x')$ in the interior of $\Xcal \times \Xcal$.

    %\item[\textbf{D5}] For all $P_n^{k(w)} \coloneqq  P_n^\infty$, (1) kernel $K$ is universal and (2) $\sup_{O \in \Ocal} p^*(O)/p_n^\infty(O) \leq c$ for some constant $c$.

    %\begin{itemize}
    %    \item The random sequence $\|h_j(\omega)\|_{j=1}^\infty$ converges monotonically to $\phi_{\h{P}}$ in $L_0^2(\h{P})$ norm. 
    %    \item The random sequence $\|h_j(w)\|_{j=1}^\infty$ and its corresponding sequence of first and second derivatives are bounded over the support $\Ocal$ for large values for $j$.
    %\end{itemize}
\end{enumerate}

These assumptions directly correspond to achieving the correct rate for the expansion provided in \ref{lemma:expension}. Assumptions \textbf{D1}, \textbf{D2} ensure that the second-order remainder term vanishes at a $1/\sqrt{n}$ rate, while Assumption \textbf{D3} guarantees the $P^*$-Donsker conditions needed for the empirical process term to vanish at the correct $1/\sqrt{n}$ rate. We stress that these assumptions are sufficient but not necessary, in that the bounded total variation condition in Assumption \textbf{D3} is one of many ways to guarantee the $P^*$-Donsker condition \footnote{In particular, estimators that satisfy the necessary rates of convergence for Assumption \textbf{D1} may not satisfy the continuous differentiability criteria of Assumption \textbf{D3}, depending on the true DGP $P^*$ and the method for the initial estimate. These assumptions are more plausible for the true distribution $P^*$ given in Section \ref{sec:sims}, as we discuss below.}. 

\paragraph{Second-Order Remainder Convergence.} As discussed in \cite{chernozhukov2017double} (amongst many other works), the first assumption \textbf{D1} corresponds to the celebrated "doubly-robust" property for the ATE functional. In particular, this assumption can be relaxed to $\|g_{P_n^0} - g_{P^*}\|_{L_2(P^*)}\times\|Q_{P_n^\infty} - Q_{P^*} \|_{L_2(P^*)} = o_P(n^{-1/2})$. Assumption \textbf{D2} is slightly different than the common \emph{positivity}/overlap assumption, in that it places an assumption on our estimated propensity $g_{P_n^0}$. In Section \ref{subsec:ate_asymp_lin}, we show how Conditions \textbf{D1}, \textbf{D2} satisfy Assumption \ref{assump:secondorderremainder}. 
%Kyra: when we are referring to a specific condition, section, assumption, we capitalize the first letter, e.g., Section 2, Condition 1, Assumption 3.

\paragraph{Pseudo Empirical Process Term Convergence.} Assumptions \textbf{D1}, \textbf{D2}, which provide sufficient conditions for Assumption \ref{assump:secondorderremainder} to hold, also satisfy the consistency requirement of Assumption \ref{assump:empprocess}, namely that $\|\phi_{P_n^\infty} -\phi_{P^*} \|_{L^2(P^*)} = o_{P^*}(1)$. We defer to works such as  \cite[Sec. 4.4]{kennedy2016semiparametric}, which demonstrates these results. Assumption \textbf{D3}  implies the main regularity condition of our work, namely that there exists a sufficiently regular sequence $\{h_j\}_{j=1}^\infty$ that converges to $\phi_{P_n^\infty}$ for all sample paths as $n \rightarrow \infty$. Assumption \textbf{D3} also places an explicit bound on the density ratio to guarantee the square integrability of $p^*/p_n^\infty$, and simplifies our analysis while satisfying the square-integrability condition of Assumption \ref{assump:S4}. The bound on the integral of the derivative guarantees the $P^*$-Donsker conditions in Assumption \ref{assump:S5}, which enables our analysis in the next section.

%Assumption \textbf{D4} closely resembles Assumption \ref{assump:S5}, but changes two requirements on sequence $\{h_j\}_{j=1}^\infty$. The first condition of \textbf{D4} is convergence with respect to the $L_0^2(\h{P})$ norm, not the $L_0^2(P^*)$ norm, and is easily satisfied by Proposition \ref{thm:mean-zero-kernel}. The second condition provides an explicit requirement on the behavior of function $h_j$ as $j \rightarrow \infty$ that satisfies the $P^*$-Donsker requirement. 

\subsection{Convergence of Pseudo Empirical Process Term}
Before delving into the von-Mises expansion of $\psi(P_n^\infty)$, we first discuss Assumption \textbf{D3}, and the importance of the $P^*$-Donsker condition. Recall that under the results of Proposition \ref{thm:mean-zero-kernel}, the RKHS $\Hcal_{P_n^\infty}$ associated with mean-zero Gaussian kernel $K_{P_n^\infty}$ is dense in $L^2_0(P_n^\infty)$ with respect to the $L^2(P_n^\infty)$ norm. Because $\phi_{P_n^\infty} \in L_0^2(P_n^\infty)$, and the RKHS $\Hcal_{P_n^\infty}$ is dense in $L^2_0(P_n^\infty)$, there must exist a sequence $\{h_j\}_{j \in \NN} \subset \Hcal_{P_n^\infty}$, where for all $\epsilon > 0$, there exists a $j(\epsilon) \in \NN$ such that for all $j > j(\epsilon)$, $\|h_j - \phi_{P_n^\infty} \|_{L^2(P_n^\infty)} < \epsilon$. Note that the existence of sequence $\{h_j\}_{j\in \NN}$ that satisfies these conditions is not due to any assumptions, but rather the set-up of the mean-zero Gaussian kernel $K_{P_n^\infty}$.

To get the desired convergence rates with respect to the true measure $P^*$, we use the first condition of Assumption \textbf{D3}, which ensures that $\sup_{O \in \Ocal} p^*
(O)/p_n^\infty(O) \leq c$ for some absolute constant $c$ for all sample paths $\omega \in \Omega$. By a simple change-of-measure with respect to a dominating measure $\lambda$, we obtain convergence results for $P^*$:
\begin{align*}
    \|h_j - \phi_{P_n^\infty}\|_{L^2(P^*)}^2 &= \int (h_j - \phi_{P_n^\infty})^2\ dP^* 
    = \int (h_j - \phi_{P_n^\infty}) (\frac{p_n^\infty}{p_n^\infty}) p^* d\lambda(O)\\
    &\leq \sup_{O \in \Ocal} |\frac{p^*}{p_n^\infty}| \times\int(h_j - \phi_{P_n^\infty})^2 dP_n^\infty(O) \\
    &\leq c \|h_j-\phi_{P_n^\infty}\|_{L^2(P_n^\infty)}^2 \quad\quad\text{(by Assumption \textbf{D3}.)}
\end{align*}
By setting $j > j(\epsilon/\sqrt{c})$, this leads to an equivalent result under $L^2(P^*)$ norm (rather than $L^2(P^\infty_n)$ norm):
\[
\|h_j - \phi_{P_n^\infty}\|_{L^2(P^*)}\leq \sqrt{c}\|h_j - \phi_{P_n^\infty}\|_{L^2(P_n^\infty)} < \epsilon.
\]
Thus, for all $\epsilon > 0$, there exists $j(\epsilon/\sqrt{c})\in \NN$ such that $j > j(\epsilon/\sqrt{c})$ implies $\|h_j - \phi_{P_n^\infty}\|_{L^2(P^*)} < \epsilon$. An immediate consequence of this result is another useful result for our analysis. By a simple application of Holder's inequality, 
\begin{align*}
|P^*(h_j - \phi_{P_n^\infty})| &\leq 
P^*[1 \times |h_j - \phi_{P_n^\infty}|]\\
&\leq P^*(|h_j-\phi_{P_n^\infty}|^2)^{1/2} \times P^*(1^2)^{1/2} \quad\quad \text{(Holder's Inequality for $p=q=2$.)}\\
&= \|h_j - \phi_{P_n^\infty} \|_{L^2(P^*)} < \epsilon.
\end{align*}
So far, using only Assumption \textbf{D3}'s condition that $\sup_{O \in \Ocal} p^*(O)/ p^\infty_n(O) \leq c$, we know that there exists a sequence $\{h_j\}_{P_n^\infty} \subset \Hcal_{P_n^\infty}$, such that for all $\epsilon >0$, there exists a $j(\epsilon/\sqrt{c}) \in \NN$ where $j > j(\epsilon/\sqrt{c})$ implies the following:
\[
\textbf{(A)}:\ \|h_j - \phi_{P_n^\infty}\|_{L^2(P^*)}< \epsilon,
\quad\quad
\textbf{(B)}:\ |P^*(h_j - \phi_{P_n^\infty})| < \epsilon.
\]
The key requirement of Assumption \textbf{D3} lies in the bounded variation criteria. While there may be many  sequences $\{h_j\}_{j\in \NN} \in \Hcal_{P_n^\infty}$ that approximate $\phi_{P_n^\infty}$ arbitrarily well, we require one such sequence $\{h_j\}_{j \in \NN}$ to satisfy the condition that for $j \geq j_1$ for some $j_1 \in \NN$, $h_j$ falls into a $P^*$-Donsker class across all sample paths $\omega \in \Omega$. To make this concrete, we first introduce well-established results by \cite{dudley_bv} and \cite{wendland_2004}.

\subsubsection{$P^*$-Donsker Conditions}
We use a simplified version of the bounded variation criterion to relate the last condition found in Assumption \textbf{D3} to $P^*$-Donsker properties:
\begin{theorem}[bounded TV and Donsker class \cite{dudley_bv}]\label{thm:tv_donsker}
A function $f$ on interval $J \subset \RR$ has its total variation defined as follows:
\[
\nu(f) \coloneqq \sup\{ \sum_{i=1}^n |f(x_i)-f(x_{i-1}) |: x_0 < x_1 < ... < x_n \in J, n \in \NN  \}.
\]
Moreover, for continuously differentiable function $f$ over a bounded support $[a,b]$, the total variation $\nu(f)$ is equivalent to $\nu(f) = \int_a^b |f'(x)| dx$. For any interval $J \subset \RR$, $M < \infty$, and probability measure $P$, $\Fcal_{M}= \{f: J \rightarrow \RR, \ \nu(f) < M\}$ is $P$-Donsker. 
\end{theorem}
We note that the discrete portion of the support $(Y,A) \in \{0,1\}^2$ can only contribute to a finite amount of variation (at most 4 distinct values), and thus we only need to consider the continuous portion of the support $\Xcal = [0,1]$, where the derivative is defined \footnote{Alternatively, we can consider the support as 4 intervals of length 1, with disconnected endpoints. This effectively encodes the the discrete support $[0,1]\times \{0,1\}^2$. If the total variation across each of these 4 intervals is bounded by some constant $M < \infty$, then the function has a total variation bound $4M+\beta$ for some fixed constant $\beta$. Thus, it suffices to consider functions $f: \Xcal \times \Acal \times \Ycal \rightarrow \RR$ as functions of simply $\Xcal$, for a fixed $(Y,A)$ pair.}. The last condition for Assumption \textbf{D3} imposes the condition that $\int_{0}^1 | \frac{\delta}{\delta x} h_j| \ dx \leq M$ for $j > j_1$, for some $j_1 \in \NN$, and therefore is equivalent to implying $h_j$ is $P^*$-Donsker for all $j > j_1$ if $\frac{\delta}{\delta x} h_j$ exists. 

Wendland \cite{wendland_2004} provides a useful result to show that $\frac{\delta}{\delta x} h_j$ not only exists, but is itself continuous:
\begin{theorem}[continuous differentiability for RKHS \cite{wendland_2004}
]\label{thm:cont_diff_rkhs}
    Let $\Xcal$ be an open subset of $\RR^q$, and let $K$ be a positive definite reproducing kernel on $\Theta$ which is $2s$ times continuously differentiable on $\Xcal$, i.e. $K\in C^{2s}(\Xcal \times \Xcal)$. Then, the associated RKHS $\Hcal_K$ is a subset of $C^s(\Xcal)$, meaning that for all $h \in \Hcal_K$, $h$ is $s$-times continuously differentiable on $\Xcal$. 
\end{theorem}
We now show this theorem directly applies by showing $K_{P_n^\infty}(O,O') \equiv K_{P_n^\infty}((x,a,y), (x',a',y')) \in C^{2}((0,1) \times (0,1))$ for fixed pairs $(a,y), (a',y') \in \{0,1\}^2$. The kernel function (parameterized with respect to $x,x'$) is as follows:
\begin{align*}
    K_{P_n^\infty}(x,x') &= \underbrace{\exp(-(x-x')^2 - \eta)}_{=f(x,x')} - \underbrace{\frac{\int \exp(-(x-x(O))^2 - \eta(O))dP_n^\infty(O) \int \exp(-(x'-x(O))^2 - \eta(O))dP_n^\infty(O)}{\int\int \exp(-\|S-T\|^2_2)dP_n^\infty(S)dP_n^\infty(T)}}_{=\frac{F(x)F(x')}{\beta}}\\
    &= f(x,x') - \frac{F(x)F(x')}{\beta}
\end{align*}
where $x(O)$ indicates the corresponding value for $x$ in $O = (x,a,y)$, $\eta = \bm{1}[y \neq y'] + \bm{1}[a \neq a'] \in \{0,1,2\}$ , $\eta(O) = \bm{1}[y\neq y(O)] + \bm{1}[a \neq a(O)] \in \{0,1,2\}$, and $\beta$ is a fixed constant that only depends on $P_n^\infty$. In this decomposition, the first term $f(x,x')$ is clearly in $C^2(\Xcal \times \Xcal)$. Thus, it remains to check that $F(x)F(x')/\beta \in C^2(\Xcal \times \Xcal)$. 

\begin{enumerate}
    \item \textbf{Continuity of First-Order Partials}: 
    To verify this, we note that the derivative of function $\exp(-(x-x(O))^2 - \eta(O))$ is bounded for all $O \in \Ocal$:
    \[|\frac{\delta}{\delta x}\exp(-(x-x(O))^2 - \eta(O))| = |-2(x-x(O))\exp(-(x-x(O))^2-\eta(O))| \leq 2, \]

    Because we obtain probability measure $0\leq P_n^\infty(O)\leq 1$ by only fitting $Q_{P_n^\infty}$, the Radon-Nikodym derivative $\frac{d P_n^\infty(O)}{d\lambda(O)} \leq 1$ (for some dominating measure $\lambda$). This permits the swap of the integral and derivative operator by the Dominated Convergence Theorem\footnote{More generally, the formal statement (Theorem 16.8, \cite{Billingsley}) requires $f(x)=\exp(-(x-x(O))^2-\eta(O))$ to be continuous with respect to $x$, measurable with respect to $O$, and locally uniformly integrably bounded. This last condition is trivially satisfied in our example by a global bound on $f(x)$ due to the $\Mcal$, and the previous conditions are satisfied by the properties of $P_n^\infty$ and the smoothness of $f(x)$. In particular, we note that the Radon-Nikodym derivative for $P_n^\infty$ need not be bounded between $[0,1]$, but any bound $M$ for our result to hold true.}:
    \begin{align*}
        \frac{\delta}{\delta x} F(x) &= \frac{\delta}{\delta x} \int\exp(-(x-x(O))^2 - \eta(O)) \ dP_n^\infty(O) = \int \frac{\delta}{\delta x}\exp(-(x-x(O))^2 - \eta(O)) \ dP_n^\infty(O)\\
        &= \int -2(x-x(O))\exp(-(x-x(O))^2-\eta(O)) dP_n^\infty(O) 
    \end{align*}
    To see that $\frac{\delta}{\delta x} F(x)$ is continuous, we note that function $g(x, x(O)) \coloneqq -2(x-x(O))\exp(-(x-x(O))^2-\eta(O))$ is clearly a continuous function, and therefore uniformly continuous with respect to $x \in [0,1]$. By definition of uniform continuity, for all $\epsilon > 0$, there exists a $\delta(\epsilon) > 0$ such that for all $x_0,x_1$ such that $|x_0-x_1| \leq \delta(\epsilon)$, $|g(x_0, x(O)) - g(x_1, x(O))| \leq \epsilon$ for fixed $(y,a), (y',a')\in \{0,1\}^2$. With the same $\delta(\epsilon)$, for any $x_0, x_1 \in \Xcal$ where $|x_0-x_1| \leq \delta(\epsilon)$, we obtain the same guarantee for $\frac{\delta}{\delta x} F(x)$:
    \begin{align*}
        |\frac{\delta}{\delta x} F(x_1) - \frac{\delta}{\delta x} F(x_0)|  &= |\int g(x_1,x(O)) dP_n^\infty(O) - \int g(x_0,x(O)) dP_n^\infty(O)|\\
        &\leq \int |g(x_1,x(O))-g(x_0, x(O))| dP_n^\infty(O)\\
        &\leq \int \epsilon \ dP_n^\infty(O) \leq \epsilon.
    \end{align*}
    Thus, we obtain that $\frac{\delta}{\delta x}F(x)$ is uniformly continuous, and $\frac{\delta}{\delta x}K_{P_n^\infty} = \frac{\delta}{\delta x}f(x,x') - [\frac{\delta}{\delta x}F(x)\times F(x')/\beta]$ is the sum of two continuous functions (symmetrically for $\frac{\delta}{\delta x'}K_{P_n^\infty}$), and therefore continuous. 
    \item \textbf{Continuity of Second-Order Partials}: We reiterate the previous steps. The second partial derivative of $\exp(-(x-x(O))^2- \eta(O))$ is also bounded and uniformly continuous:
    \begin{align*}
       \frac{\delta^2}{\delta^2 x} \exp(-(x-x(O))^2- \eta(O))
      &= 4(x-x(O))\exp(-(x-x(O))^2 \\
      &\quad+ \eta(O))
      + 4(x-x(O))^2\exp(-(x-x(O))^2 - \eta(O)) \\
      &= 4(x-x(O))\exp(-(x-x(O))^2-\eta(O))(1+x-x(O))
    \end{align*}
    For all $O \in \Ocal$, $|\frac{\delta^2}{\delta^2 x} \exp(-(x-x(O))^2- \eta(O))| \leq 8$, and therefore by dominated convergence, we obtain the second partial derivative of $F(x)$ as the following:
    \[
    \frac{\delta^2}{\delta^2 x} F(x) = \int 4(x-x(O))\exp(-(x-x(O))^2-\eta(O))(1+x-x(O)) dP_n^\infty(O)
    \]
    Because $4(x-x(O))\exp(-(x-x(O))^2-\eta(O))(1+x-x(O))$ is a uniformly continuous function with respect to $x$ on $\Xcal$, we know $\frac{\delta}{\delta^2 x}F(x)$ is also uniformly continuous, and therefore $\frac{\delta^2}{\delta^2 x} K_{P_n^\infty} = \frac{\delta^2}{\delta^2 x} f(x,x') + (\frac{\delta^2}{\delta^2 x} F(x))\frac{F(x')}{\beta}$ is (uniformly) continuous. This holds symmetrically for $\frac{\delta^2}{\delta^2 x'} K_{P_n^\infty}$. 

    \item \textbf{Continuity of Cross Partials}: 
    Lastly, the cross partial derivative $\frac{\delta^2}{\delta x\delta x'} K_{P_n^\infty}$ also continuous, as shown below: 
    \[\frac{\delta^2}{\delta x \delta x'} K_{P_n^\infty} = \frac{\delta^2}{\delta x \delta x'}f(x,x')- \frac{\delta}{\delta x}F(x) \times \frac{\delta}{\delta x}F(x')/ \beta.\]
    We have already shown that $\frac{\delta}{\delta x}F(x), \frac{\delta}{\delta x'}F(x')$ are continuous with respect to $x,x'$ respectively, and $\frac{\delta^2}{\delta x \delta x'} f(x,x')$ is continuous with respect to $x,x'$. Thus,  $\frac{\delta}{\delta x \delta x'}K_{P_n^\infty}$ must be continuous with respect to $\Xcal \times \Xcal$.
\end{enumerate}
By the smoothness of its partial derivatives, $K_{P_n^\infty} \in C^{2}(\Xcal \times \Xcal)$, and therefore for all $h \in \Hcal_{P_n^\infty}$, the derivative $\frac{\delta}{\delta x} h(x)$ exists and is continuous. Thus, for the sequence $\{h_j\}_{j \in \NN} \subset \Hcal$, $|\frac{\delta}{\delta x} h_j|$ is well defined for all $j \in \NN$. To satisfy the $P^*$-Donsker condition, we use the condition given by Theorem \ref{thm:tv_donsker}, which is $\int |\frac{\delta}{\delta x} h_j(x)| dx \leq M$ for across all $(y,a)\in \{0,1\}^2$ for some universal constant $M$ when $j \geq j_1$ (across all sample paths $\omega \in \Omega$). 

 k\paragraph{Main Implication of $P^*$-Donsker Property} To leverage the key lemma involving the $P^*$-Donsker condition, we first note that $\|\phi_{P_n^\infty} - \phi_{P^*}\|_{L^2(P^*)}^2 = o_{P^*}(1)$ by Assumptions \textbf{D1} and \textbf{D2} \footnote{For a more detailed derivation, please refer to Page 22 of \cite{kennedy2023}.}. By setting $j^* \geq \max(j_1, j(\frac{1}{\sqrt{nc}}))$, we obtain the desired consistency result via Property \textbf{(A)}:
\begin{align*}
   \|h_{j^*} - \phi_{P^*}\|_{L^2(P^*)}^2 &\leq 
    \|h_{j^*} - \phi_{P_n^\infty}\|_{L^2(P^*)}^2 + 
    \|\phi_{P_n^\infty} - \phi_{P^*}\|_{L^2(P^*)}^2 \\
    &\leq c(\frac{1}{nc}) + o_{P^*}(1) = o_{P^*}(1)
\end{align*}
Thus, $h_{j^*}$ is a consistent estimator of $\phi_{P^*}$. Furthermore, because $j^*\geq j_1$, $\int_0^1 |\frac{\delta}{\delta x}h_j| dx \leq M$, and thus $h_j$ falls into a $P^*$-Donsker class by Assumption \textbf{D3} and Theorem \ref{thm:tv_donsker}. An immediate implication of these results is as follows:

\begin{lemma}[Lemma 19.24, van der Vaart (2000)]\label{lemma:donsker_emp}
    Suppose that $\Fcal$ is a $P$-Donsker class of measurable functions and $\h{f}_n$ is a sequence of random functions that take their values in $\Fcal$ such that $\int (\h{f}_n(x) - f_0(x))^2 dP(x) \rightarrow 0$ for some $f_0 \in L^2(P)$. Then, $\sqrt{n}(\PP_n-P)(\h{f}_n-f_0) = o_{P^*}(1)$, or equivalently, $(\PP_n-P)(\h{f}_n- f_0) = o_{P^*}(1/\sqrt{n})$.
\end{lemma}

Our function $h_{j^*} = h_{j(\frac{1}{\sqrt{nc}})}$ is a consistent estimator of $\phi_{P^*} \in L^2(P^*)$, and satisfies the $P^*$-Donsker condition. By Lemma \ref{lemma:donsker_emp}, this immediately implies that the term $(\PP_n-P^*)(h_{j^*}- \phi_{P^*}) = o_{P^*}(1/\sqrt{n})$, which enables the asymptotic linearity of our estimator. Putting all conditions of Assumption \textbf{D1-3} together, there exists a sequence $\{h_j\}_{j\in \NN}$ that satisfies all of the following criteria for $h_j$, where $j^* \geq \max(j_1, j(\frac{1}{n\sqrt{c}}))$:
\begin{align*}
&\textbf{(A)}:\ \|h_{j^*} - \phi_{P_n^\infty}\|_{L^2(P^*)} < 1/n = o_{P^*}(1/\sqrt{n}),\\
&\textbf{(B)}:\ |P^*(h_{j^*} - \phi_{P_n^\infty})| < 1/n = o_{P^*}(1/\sqrt{n}),\\
&\textbf{(C)}:\ (\PP_n-P^*)(h_{j^*}- \phi_{P^*}) = o_{P^*}(1/\sqrt{n})
\end{align*}
Note that \textbf{(A)}, \textbf{(B)} are implied by Assumption \textbf{D3}'s condition on the density ratio, while \textbf{(C)} is the result of Assumption \textbf{D3}'s condition on the behavior of $\{h_j\}_{j \in \NN}$ and Assumptions \textbf{D1}, \textbf{D2}. Below, we show the desired $o_{P^*}(1/\sqrt{n})$ rate for the pseudo-empirical process term, using properties \textbf{(B)}, \textbf{(C)}, and Assumption \ref{assump:S3} (convergence in the interior of the model). 

\subsubsection{Convergence Rates for the Pseudo-Empirical Process Term}
We turn our attention to proving the $o_{P^*}(1/\sqrt{n})$ rate for Term $(a)$ in the Equation \eqref{eq:ate_theory_expansion}. Note that under Assumption \ref{assump:S3}, $\PP_n h =0$ for every $h \in \Hcal_{P_n^\infty}$, giving us the following equality:
\[(a)= - \PP_n(\phi_{P_n^\infty})+ (\PP_n-P^*)(\phi_{P_n^\infty}-\phi_{P^*})= - \PP_n({-h_{j^*}}+\phi_{P_n^\infty})+ (\PP_n-P^*)(\phi_{P_n^\infty}-\phi_{P^*}).\]

Given property \textbf{(B)}, we can rewrite the "pseudo-empirical process term" $(a)$ as follows:
\begin{align*}
    (a) &= -\PP_n(\phi_{P_n^\infty}-h_{j^*}) + (\PP_n-P^*)(\phi_{P_n^\infty}-\phi_{P^*}) \\
    &= -\PP_n(\phi_{P_n^\infty}-h_{j^*}) + (\PP_n-P^*)(\phi_{P_n^\infty}-\phi_{P^*}) + P^*(\phi_{P_n^\infty} - h_{j^*}) \underbrace{-P^*(\phi_{P_n^\infty} - h_{j^*})}_{=\pm o_{P^*}(1/\sqrt{n})}\\
    &=-[\PP_n(\phi_{P_n^\infty})-P^*(\phi_{P_n^\infty})] + [\PP_n(h_{j^*})-P^*(h_{j^*})] + (\PP_n-P^*)(\phi_{P_n^\infty}-\phi_{P^*})  \pm o_{P^*}(1/\sqrt{n})\\
    &=(\PP_n-P^*)(h_{j^*}-\phi_{P^*})  \pm o_{P^*}(1/\sqrt{n}).\label{eq:(a)}
\end{align*}
Using Property \textbf{(C)}, we conclude that $(\PP_n-P^*)(h_{j^*}- \phi_{P^*}) = o_{P^*}(1/\sqrt{n})$, and thus we obtain that $(a) = o_{P^*}(1/\sqrt{n})$. 

\subsection{Convergence of Second-Order Remainder Term}\label{app:sor}
We first rewrite $R_2(P_n^\infty, P^*) = (b)$ in Equation \eqref{eq:ate_theory_expansion} using the analytic form of $\phi_{P}$. By our set-up in Section \ref{sec:sims}, $P_n^\infty = \PP_n(X) \times P_n^0(A|X)\times P_n^\infty(Y|A,X)$,
yielding: 
% which gives us the following form:
\begin{align*}
    R_2(P_n^\infty, P^*) &= \psi(P_n^\infty) - \psi(P^*) + P^*[\phi_{P_n^\infty}]\\
    &= \psi(P_n^\infty) + \psi(P^*) + P^*\Bigg[\left(\frac{\mathbbm{1}_1(A)}{g_{P_n^0}(X)}-\frac{\mathbbm{1}_0(A)}{1-g_{P_n^0}(X)}\right)
   (Y-Q_{P_n^\infty}(A,X)) \\ 
   & \quad + (Q_{P_n^\infty}(1,X)-Q_{P_n^\infty}(0,X)-\PP_n[Q_{P_n^\infty}(1,X)-Q_{P_n^\infty}(0,X)]) \Bigg]\\
   &= R_2^1(P_n^\infty, P^*) - R_2^0(P_n^\infty,  P^*),
\end{align*}
where $R_2^1(P_n^\infty, P^*), R_2^0(P_n^\infty,  P^*)$ are defined as follows:
\begin{align*}
    R_2^1(P_n^\infty, P) &= \mu_1(P_n^\infty) - \mu_1(P^*) \\
    &+ P^*\left[\frac{\mathbbm{1}_1(A)}{g_{P_n^0}(X)}[Y-Q_{P_n^\infty}(1,X)\right] + Q_{P_n^\infty}(1,X)-\PP_n[Q_{P_n^\infty}(1, X)]],\\
% \end{align*}
% \begin{align*}
    R_2^0(P_n^\infty, P^*) &= \mu_0(P_n^\infty) - \mu_0(P^*)\\
    &+ P^*\left[\frac{\mathbbm{1}_0(A)}{1-g_{P_n^0}(X)}[Y-Q_{P_n^\infty}(0,X)\right] + Q_{P_n^\infty}(0,X) - \PP_n[Q_{P_n^\infty}(0,X)]],
\end{align*}
with $\mu_a(P)=  P_X[P_{Y|A,X}[Y|A=a,X]]$ such that $\psi(P) = \mu_1(P)-\mu_0(P)$. Thus, it suffices to show that $R_2^1(P_n^\infty, P^*), R_2^0(P_n^\infty, P^*)$ are $o_{P^*}(1/\sqrt{n})$ under our assumptions. We begin with $R_2^1(P_n^\infty, P^*)$.  Our term $R_2^1(P_n^\infty, P)$ reduces to the following form:
\begin{align*}
     R_2^1(P_n^\infty, P^*) &= \mu_1(P_n^\infty) - \mu_1(P^*)\\
     &\quad + P^*\left[\frac{\mathbbm{1}_1(A)}{g_{P_n^0}(X)}[Y-Q_{P_n^\infty}(1,X)] + Q_{P_n^\infty}(1,X)-\PP_n[Q_{P_n^\infty}(1, X)]\right]\\
     &=\mu_1(P_n^\infty)- \mu_1(P^*) \\
     &\quad + P^*\left[\frac{\mathbbm{1}_1(A)}{g_{P_n^0}(X)}[Y-Q_{P_n^\infty}(1,X)] + Q_{P_n^\infty}(1,X)\right] - P^*\big[\underbrace{\mu_1(P_n^\infty)}_{=\PP_n[Q_{P_n^\infty}(1,X)]}\big]\\
     &= -\mu_1(P^*)  + P^*\left[\frac{\mathbbm{1}_1(A)}{g_{P_n^0}(X)}[Y-Q_{P_n^\infty}(1,X)] + Q_{P_n^\infty}(1,X)\right]\\
     &= -\mu_1(P^*) + P^*\left[\frac{\mathbbm{1}_1(A)}{g_{P_n^0}(X)}Y\right]- P^*\left[\frac{\mathbbm{1}_1(A)}{g_{P_n^0}(X)}Q_{P_n^\infty}(1,X)\right] + P^*[Q_{P_n^\infty}(1,X)]\\
     &= P^*_X\left[Q_{P^*}(1,X) - Q_{P_n^{\infty}}(1,X)\right] + \underbrace{P^*\left[\frac{\mathbbm{1}_1(A)}{g_{P_n^0}(X)}Y\right]}_{=(c)}- \underbrace{P^*\left[\frac{\mathbbm{1}_1(A)}{g_{P_n^0}(X)}Q_{P_n^\infty}(1,X)\right]}_{=(d)}.
\end{align*}
For term $(c)$, we can re-express this as the following:
\begin{align*}
    P^*\left[\frac{\mathbbm{1}_1(A)}{g_{P_n^0}(X)}Y\right] &= 
    P^*_{X}\left[P^*_{Y,A|X}\left[\frac{\mathbbm{1}_1(A)}{g_{P_n^0}(X)}Y|X\right]\right]
    = P^*_{X}\left[\frac{1}{{g_{P_n^0}(X)}}P^*_{Y,A|X}[\mathbbm{1}_1(A)Y|X]\right]\\
    &= P^*_{X}\left[\frac{1}{{g_{P_n^0}(X)}} \ \underbrace{P^*_{Y,A|X} [\mathbbm{1}_1(A)|X]}_{= g_{P^*(X)}} \ P^*_{Y|A,X}[Y\ |\ X,A=1]\right]\\
    &= P_X^{*}\left[\frac{ g_{P^*}(X) }{g_{P_n^0}(X)} Q_{P^*}(1,X)\right].
\end{align*}
Using the same steps, we obtain that term $(d)= P_X^{*}\left[\frac{ g_{P^*}(X) }{g_{P_n^0}(X)} Q_{P_n^\infty}(1,X)\right]$. Thus, $R_2^1(P_n^\infty, P^*)$ takes the following form:
\begin{align*}
    R_2^1(P_n^\infty, P^*) &= P^*_X\left[Q_{P^*}(1,X) - Q_{P_n^{\infty}}(1,X)\right] + P^*_X\left[\frac{g_{P^*}(X)}{g_{P_n^0}(X)} * \left[Q_{P^*}(1,X)-Q_{P_n^\infty}(1,X)\right]\right]\\
    &= P^*_X\left[\frac{g_{P^\infty_n}(X)}{g_{P^\infty_n}(X)}\left[Q_{P^*}(1,X) - Q_{P_n^{\infty}}(1,X)\right] \right] \ + \\
    &\quad P^*_X\left[\frac{g_{P^*}(X)}{g_{P_n^0}(X)}  \left[Q_{P^*}(1,X)-Q_{P_n^\infty}(1,X)\right]\right]\\
    &= P^*_X\left[\frac{1}{g_{P_n^0}(X)}(g_{P_n^0}(X)- g_{P^*}(X))\times(Q_{P^*}(1,X)-Q_{P_n^\infty}(1,X))\right]\\
    &\leq \sup_{x \in X}\frac{1}{g_{P_n^0}(X)}\|g_{P_n^0}-g_{P^*}\|_{L_2(P^*)}\|Q_{P^*}(1, \cdot)- Q_{P_n^\infty}(1, \cdot) \|_{L_2(P^*)}.
\end{align*}
Then, under our assumptions that $\|g_{P_n^0} - g_{P^*}\|_{L_2(P^*)}$ and $\|Q_{P_n^\infty} - Q_{P^*}\|_{L_2(P^*)}$ are $o_{P^*}(n^{-1/4})$ (Assumption \textbf{D1}) and $g_{P_n^0} \geq c$ (Assumption \textbf{D2}), we have the desired result:
\[R_2^1(P_n^\infty, P^*) \leq \frac{1}{c} o_{P^*}(n^{-1/4})  o_{P^*}(n^{-1/4}) = o_{P^*}(n^{-1/2}).\]
The proof for $R_2^0(P_n^\infty, P^*)$ follows the same exact steps as above, so we omit it here for brevity. Together, we obtain:
% Thus, we get the desired result:
\[
R_2(P_n^\infty, P^*) = R_2^1(P_n^\infty, P^*)- R_2^0(P_n^\infty, P^*) =o_P(1/\sqrt{n})-o_P(1/\sqrt{n}) =o_P(1/\sqrt{n}).
\]
